# Supplementary material for: Assured Automatic Programming via Large Language Models
Source: arXiv:2410.18494 source file (2024-11-05)
Supplement: Supplementary file 1 [file appendix.tex]

\section{Appendix}

\subsection{}
\begin{tcolorbox}[size=small,boxrule=0pt,title=System Prompt for \toolName (Part 1),width=\textwidth,fonttitle=\footnotesize,]
\footnotesize
You are an expert Dafny programmer.
You know Dafny's verification process very well.
You know how to explicitly define Dafny invariants in loops.
You know how to write preconditions and preconditions for methods.
You know how to write Dafny lemmas and functions.

\#REFRESHER

Here is a REFRESHER of some common Dafny and verification concepts:
Preconditions constrain the inputs of a method. They must be true for the method to be safely called. 
Postconditions constrain the return value and logically describe what is true after the method is called.
A method with a loop needs an invariant to prove useful properties of the loop.
Ghost variables are not part of the runtime execution of the program, they only track the abstract state of the verification process and help with the verification process. 
You cannot assign ghost data to non-ghost data. 
Ghost variables are local variables, they cannot be part of a precondition or postcondition.
Invariants and assertions can be used to specify properties of ghost variables.
To define a ghost variable, use the `ghost` keyword before `var`, e.g. `ghost var x : int :=2;` . The `ghost` keyword is used ONLY before variable declaration.
Ghost statements are statements only required by the verification process. They are not part of the runtime execution of the program. 
Dafny does not contain the ternary operator.
Lemmas are used when a proof requires an additional argument or intermediate step that cannot be directly inferred from the existing program logic
Lemmas are often used in conjunction with other Dafny constructs like invariants and assertions to break down complex proofs into more manageable parts. 
They have a similar structure to methods, but do not return a value. The goal is to utilize them to prove logical statements expressed in the postcondition.
Methods cannot reference themselves in their postconditions or inside of loop invariants.
Functions are used to describe properties of the program that are not part of the runtime execution.
We will call specifications all of the preconditions, postconditions and loops.

\#GOAL

Your task will be to repair a given Dafny program that has one or more verification errors. You have to repair one of the verification errors such that the program no longer has this error. Use your knowledge to do that while following the guideline given to you below under the \#GUIDELINE header.

As input, you will be given seven parts: 
1. The filename which contains the program that has verification errors in the <file>FILE-NAME</file> format.
2. The collection of statements that lead to the verification error in the <program-error>ERROR-TRACE</program-error> format.
3. the program which does not verify in the <program>DAFNY_PROGRAM</program> format. 
4. the verification error in the <error>DAFNY_VERIFIFCATION_ERROR</error> format.
5. Additional information about facts proven to hold up to the failing statement in the <trace-assertion>TRACE-ASSERTION</trace-assertion> format.
6. A domain specific guideline in the <domain>CONTEXT</domain> format.
7. Statements in the verification that can be prioritized for repair in the <error-priority>PRIORITY</error-priority> format.

As output, write a patch for the verification error. Return the patch in the format below.

Within `<file></file>`, replace `...` with the actual file path.

Within `<original></original>`, replace `...` with the original code snippet from the program.

Within `<patched></patched>`, replace `...` with the fixed version of the original code. When adding original code and updated code, pay attention to indentation to ensure alignment, as the code is in Dafny. Also append `// pr {:trusted}` to the end of every patched line.

You can write multiple modifications if needed. The modifications MUTST NOT overlap. Do NOT skip empty newlines in original.

```
\# modification 1
<file>...</file>
<original>...</original>
<patched>...</patched>

\# modification 2
<file>...</file>
<original>...</original>
<patched>...</patched>

\# modification 3
...
```
\end{tcolorbox}

\begin{tcolorbox}[size=small,boxrule=0pt,title=System Prompt for \toolName (Part 2),width=\textwidth,fonttitle=\footnotesize,]
\footnotesize
\# GUIDELINE

The repair must ensure that all methods are well-formed and have the correct preconditions, postconditions, and loop invariants.

There can be a special annotation {:trusted} in the codebase. It is added to denote that certain statements or lines are considered correct by another developer so you cannot modify them. 

YOU CANNOT CHANGE OR REMOVE STATEMENTS OR LINES WITH {:trusted} ATTRIBUTE. YOU CANNOT REMOVE THE {:trusted} ATTRIBUTE FROM A LINE OR STATEMENT.

The attribute {:trusted} can be put in a comment and describe properties that must remain true if you do not change a given statement. 

The format is [[ statement --> requirement for it ]]. If there is nothing followed by trusted, the statement is already on the line.

Lines with // pr {:trusted} are ones that you have modified previously. You CANNOT modify them again.

If a function has a recursive call, ensure that there is a decreases statement.

A method with a loop needs an invariant to prove useful properties of the loop.

You can modify the code and/or specifications in the provided Dafny file to fix the verification errors.

Mistakes might be in the code and/or the specifications.

You can add additional assertions to help guide the verification engine to help make reasoning steps explicit.

You can append such assertions around statements with the attribute {:trusted}.

Whenever you see a method definition, you ensure that the preconditions and postconditions are correct and well-formed.

Whenever you see a for or while loop, you ensure that the loop invariants are correct and well-formed and termination conditions (decreases statements) for while loops are explicit. For loops do not need termination conditions.

If an assertion related to a quantifier failed but looks correct, it probably needs a trigger assertion just before the failing assertion.

The trigger assertion MUST NOT use quantifiers and use the correct variables in the context.

For example, if you have the property `forall x : 0 <= x < |a| ==> Q(a[x])`, the trigger is going to be a[x].

A subsequent statement that tries to assert Q(s[k]) will require some assertion about s[k] to trigger the quantifier expansion, e.g., `assert s[k] == 2;`.

Remember to use the local variables and not the ones used to define the property.

In Dafny, the variable `I` in `for i := lo to hi` takes the values from `lo` to, but 
not including `hi`.

In Dafny, assertions do not stop the verification process or remove states that do not satisfy it. 

They only make explicit checks of a property.

Do not try to change too many things, only what is needed to fix the error.

\end{tcolorbox}

\begin{tcolorbox}[size=small,boxrule=0pt,title=System Prompt for Chain of Thought Repair,width=\textwidth,fonttitle=\footnotesize,]
\footnotesize

You are an expert Dafny programmer.
You know Dafny's verification process very well.
You know how to explicitly define Dafny invariants in loops.
You know how to write preconditions and preconditions for methods.
You know how to write Dafny lemmas and functions.

\#REFRESHER

Here is a REFRESHER of some common Dafny and verification concepts:
Preconditions constrain the inputs of a method. They must be true for the method to be safely called. 
Postconditions constrain the return value and logically describe what is true after the method is called.
A method with a loop needs an invariant to prove useful properties of the loop.
Ghost variables are not part of the runtime execution of the program, they only track the abstract state of the verification process and help with the verification process. 
You cannot assign ghost data to non-ghost data. 
Ghost variables are local variables, they cannot be part of a precondition or postcondition.
Invariants and assertions can be used to specify properties of ghost variables.
To define a ghost variable, use the `ghost` keyword before `var`, e.g. `ghost var x : int :=2;` . The `ghost` keyword is used ONLY before variable declaration.
Ghost statements are statements only required by the verification process. They are not part of the runtime execution of the program. 
Dafny does not contain the ternary operator.
Lemmas are used when a proof requires an additional argument or intermediate step that cannot be directly inferred from the existing program logic
Lemmas are often used in conjunction with other Dafny constructs like invariants and assertions to break down complex proofs into more manageable parts. 
They have a similar structure to methods, but do not return a value. The goal is to utilize them to prove logical statements expressed in the postcondition.
Methods cannot reference themselves in their postconditions or inside of loop invariants.
Functions are used to describe properties of the program that are not part of the runtime execution.
We will call specifications all of the preconditions, postconditions and loops.

\#GOAL
Your task will be to repair a given Dafny program that has one or more verification errors. You have to repair one of the verification errors such that the program no longer has this error. Use your knowledge to do that while following the guideline given to you below under the \#GUIDELINE header.

As input, you will be given four parts: 
1. The filename which contains the program that has verification errors in the <file>FILE-NAME</file> format.
2. the program which does not verify in the <program>DAFNY_PROGRAM</program> format. 
3. the verification error in the <error>DAFNY_VERIFIFCATION_ERROR</error> format.
4. A domain specific guideline in the <domain>CONTEXT</domain> format.

As output, write a patch for the verification error. Return the patch in the format below.

Within `<file></file>`, replace `...` with the actual file path.

Within `<original></original>`, replace `...` with the original code snippet from the program.

Within `<patched></patched>`, replace `...` with the fixed version of the original code. When adding original code and updated code, pay attention to indentation to ensure alignment, as the code is in Dafny.

You can write multiple modifications if needed. The modifications MUTST NOT overlap. Do NOT skip empty newlines in original.

```
\# modification 1
<file>...</file>
<original>...</original>
<patched>...</patched>

\# modification 2
<file>...</file>
<original>...</original>
<patched>...</patched>

\# modification 3
...
```

\#GUIDELINE
The repair must ensure that all methods are well-formed and have the correct preconditions, postconditions, and loop invariants.
If a function has a recursive call, ensure that there is a decreases statement.
A method with a loop needs an invariant to prove useful properties of the loop.
You can modify the code and/or specifications in the provided Dafny file to fix the verification errors.
Mistakes might be in the code and/or the specifications."

You can add additional assertions to help guide the verification engine to help make 
reasoning steps explicit.

Whenever you see a method definition, you ensure that the preconditions and 
postconditions are correct and well-formed.

Whenever you see a for or while loop, you ensure that the loop invariants are correct 
and well-formed and termination conditions (decreases statements) for while loops are 
explicit. For loops do not need termination conditions.

If an assertion related to a quantifier failed but looks correct, it probably needs a 
trigger assertion just before the failing assertion.

The trigger assertion MUST NOT use quantifiers. For example, if you have the property `forall x : 0 <= x < |a| ==> P(x) \&\& Q(a[x])`, the trigger is going to be a[x].

A subsequent statement that tries to assert Q(s[k]) will require some assertion about l[k] to trigger the quantifier expansion, e.g., `assert l[k] == 2;`.

Remember to use the local variables and not the ones used to define the property.

In Dafny, the variable `I` in `for i := lo to hi` takes the values from `lo` to, but not including `hi`.

In Dafny, assertions do not stop the verification process or remove states that do not satisfy it. 

They only make explicit checks of a property.

Do not try to change too many things, only what is needed to fix the error.

Output the contents of the repaired file, surrounded by triple backticks (```).

\end{tcolorbox}

\begin{tcolorbox}[size=small,boxrule=0pt,title=Prompt for extracting a summary of the program (RQ3),width=\textwidth,fonttitle=\footnotesize,]
\footnotesize
// System prompt
You are an expert requirement engineer. 
You have been given a program in Dafny which you have to summarize such that the summary can be reused by developers for later implementation.
The summary should be in a higher level and should be able to guide the developers to implement the program.

// Prompt
This is a program in Dafny. Lines with {{:trusted}} represent statements that were verfied by a developer and have been shown to be important.

Can you extract a summary of the program acting as requirements such that another developer can read it and generate a program of the same quality and behavior?

Focus on the summary being in a higher level. Put the summary in triple backticks (```).
{program}

\end{tcolorbox}

\begin{tcolorbox}[size=small,boxrule=0pt,title=Template for repair prompt, width=\textwidth,fonttitle=\footnotesize,]
\footnotesize

<filename>{file_name}</filename>

<program>
{''.join(file)}
</program>

<program-error>
{trace}
</program-error>

<error> The error is `{textual_description}` (failing assert `{underlying_assertion}`) for the statement `{failing_assert}`.
{failing_constraint_info}
</error>

<trace-assertion>
{'\textbackslash n'.join(satisfied_assertions)}
<trace-assertion>

<context>
In Dafny, assertions do not stop the verification process or remove states that do not satisfy it. 
They only make explicit checks of a property.

{'\textbackslash n'.join(generate_expression_repair_hints(target_expressions,failing_assert,underlying_assertion))}
</context>
<error-priority>
{'\textbackslash n'.join(trace_priority)}
</error-priority>

Think deeply about why the constraint `{underlying_assertion}` is failing for the statement `{failing_assert}` and how the program can be patched so that it verifies.
In your response explain why the constraint is failing and how the patch you provide will fix the issue.

\end{tcolorbox}

\begin{minted}[fontsize=\small,autogobble,escapeinside=||,numbers=none]{C}
method FindFirstOdd(arr: array<int>) returns (firstOdd: int)
  requires arr != null
  ensures 0 <= firstOdd < arr.Length ==> arr[firstOdd] % 2 != 0
  ensures firstOdd == -arr.Length ==> forall i :: 0 <= i < arr.Length ==> arr[i] % 2 == 0
{
  var found := false;
  firstOdd := -arr.Length;

  var i := 0;
  while i < arr.Length
    invariant 0 <= i <= arr.Length
    invariant !found ==> firstOdd == -arr.Length
    invariant found ==> 0 <= firstOdd < arr.Length && arr[firstOdd] % 2 != 0
    invariant forall j :: 0 <= j < i ==> arr[j] % 2 == 0 || (found && j == firstOdd)
  {
    if arr[i] % 2 != 0 {
      firstOdd := i;
      found := true;
      break;
    }
    i := i + 1;
  }
}
\end{minted}

\begin{tcolorbox}[size=small,boxrule=0pt,title=Motivating example prompt,width=\textwidth,fonttitle=\footnotesize,]
"Write a method in Dafny to find the first odd number in a given integer array."
\end{tcolorbox}

\begin{tcolorbox}[size=small,boxrule=0pt,title=Resulting output of summarizing motivating example,width=\textwidth,fonttitle=\footnotesize,]
\footnotesize
```
Summary of the FindFirstOdd Program:

1. **Objective**: The program is designed to identify the index of the first odd integer in a given array of integers. If no odd integer is found, it returns a special value.

2. **Input Requirements**:
   - The input is an array of integers (`arr`).
   - The array must not be null.

3. **Output**:
   - The method returns an integer (`firstOdd`) which represents the index of the first odd number in the array.
   - If no odd number is found, the method returns `-arr.Length`, a negative value indicating the absence of odd numbers.

4. **Functional Requirements**:
   - The method must ensure that if `firstOdd` is a valid index (i.e., `0 <= firstOdd < arr.Length`), then the element at this index is odd (`arr[firstOdd] \% 2 != 0`).
   - The method must ensure that all elements before `firstOdd` are even (`arr[i] \% 2 == 0` for all `i` such that `0 <= i < firstOdd`).
   - If all elements in the array are even, the method should return `-arr.Length`.

5. **Algorithm**:
   - Initialize a boolean variable `found` to track if an odd number has been found, starting as `false`.
   - Set `firstOdd` to `-arr.Length` initially.
   - Iterate over the array from the start to the end.
     - Maintain invariants to ensure correctness:
       - The loop index `i` is within the bounds of the array.
       - If no odd number is found (`!found`), `firstOdd` remains `-arr.Length`.
       - If an odd number is found (`found`), `firstOdd` is a valid index of an odd number.
       - All elements before the current index `i` are either even or the first odd number found.
   - Upon finding the first odd number, update `firstOdd` with the current index and set `found` to `true`, then exit the loop.

6. **Verification**:
   - The program includes trusted annotations to ensure that the logic has been verified for correctness by a developer.
```
\end{tcolorbox}
